# Supplementary material for: Physical 3D Adversarial Attacks against Monocular Depth Estimation in Autonomous Driving
Source: arXiv:2403.17301 source file (2024-03-27)
Supplement: Supplementary file 1 [file X_suppl.tex]

\clearpage
\setcounter{page}{1}
\maketitlesupplementary

\appendix
\section{Implementation Details}
\subsection{Experimental Settings}

\hspace{1em}\textbf{Scenes.} We generate the datasets for training and evaluating attack methods using the Carla simulator. For autonomous driving scenarios, we selected a variety of background environments, including urban roads, highways, country roads, etc. To improve attack robustness in bad weather conditions, we choose four kinds of weather: foggy, rainy, sunny, and cloudy. The parameter settings for controlling the weather in CARLA are shown in Table~\labelcref{tab5}.

\begin{table}[!t]
\caption{Weather parameter settings in Carla to simulate cloudy, sunny, rainy, and foggy.}
\label{tab5}
  \centering
  \captionsetup{skip=3pt}
\resizebox{\linewidth}{!}{
  \begin{tabular}{ccccc}
    \toprule
    \multirow{2}[3]{*}{Parameters} & \multicolumn{4}{c}{Weather conditions}\\
\cmidrule{2-5}          & cloudy & sunny & rainy & foggy\\
    \midrule
    sun\_azimuth\_angle & 300 & 300 & -1 & 300\\
    sun\_altitude\_angle & 45 & 90 & 45 & 45\\
    cloudiness & 30 & 10 & 100 & 100\\
    precipitation & 0 & 0 & 100 & 0\\
    precipitation\_deposits & 0 & 0 & 90 & 0\\
    fog\_density & 1 & 0 & 3 & 15\\
    \bottomrule
  \end{tabular}
}
\end{table}

\textbf{Cars.} We select multiple types of cars in the Carla simulator. Lincoln MKZ2017, Seat Leon, Audi Etron, and Citreon C3 are four types of cars used for effectiveness and robustness evaluation. Additionally, Tesla Model 3 is used for ablation studies. All these cars are visualized in Figure~\labelcref{fig:11}.

\begin{figure}[!t]
    \centering
    \includegraphics[width=\columnwidth]{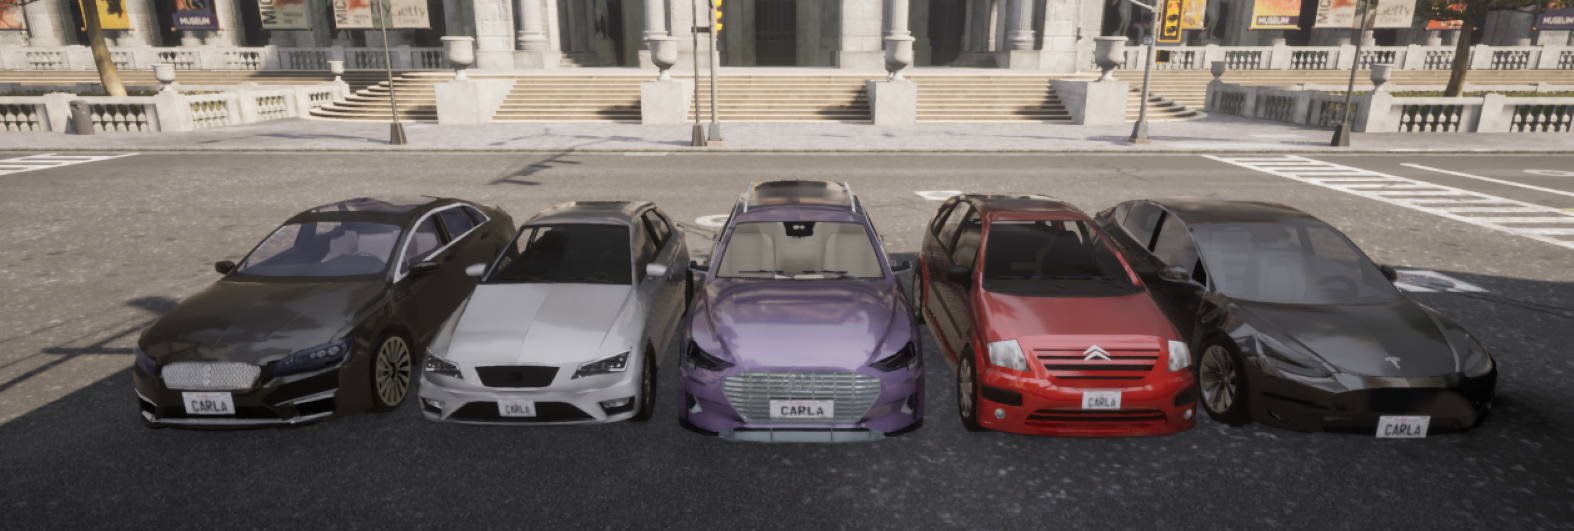}
    \caption{Five types of cars used in our evaluations.}
    \label{fig:11}
\end{figure}

\textbf{Camera settings.} For attack robustness, we take images with the RGB camera sensor in Carla at a random angle of 0-360$^{\circ}$, within a 3-15m distance range and a 0.5-2m height range, as shown in Figure~\labelcref{fig:12}. We take 8400 photo-realistic images for attack texture generation (210 scenes $\times$ 4 weather conditions $\times$ 10 camera positions). For a single texture evaluation, we take a total of 6124 images (discrete part: 30 scenes $\times$ 4 weather conditions $\times$ 10 camera positions $\times$ 4 cars, and continuous part: 4 weather conditions $\times$ 331 frames).

\begin{figure}[!t]
    \centering
    \includegraphics[width=\columnwidth]{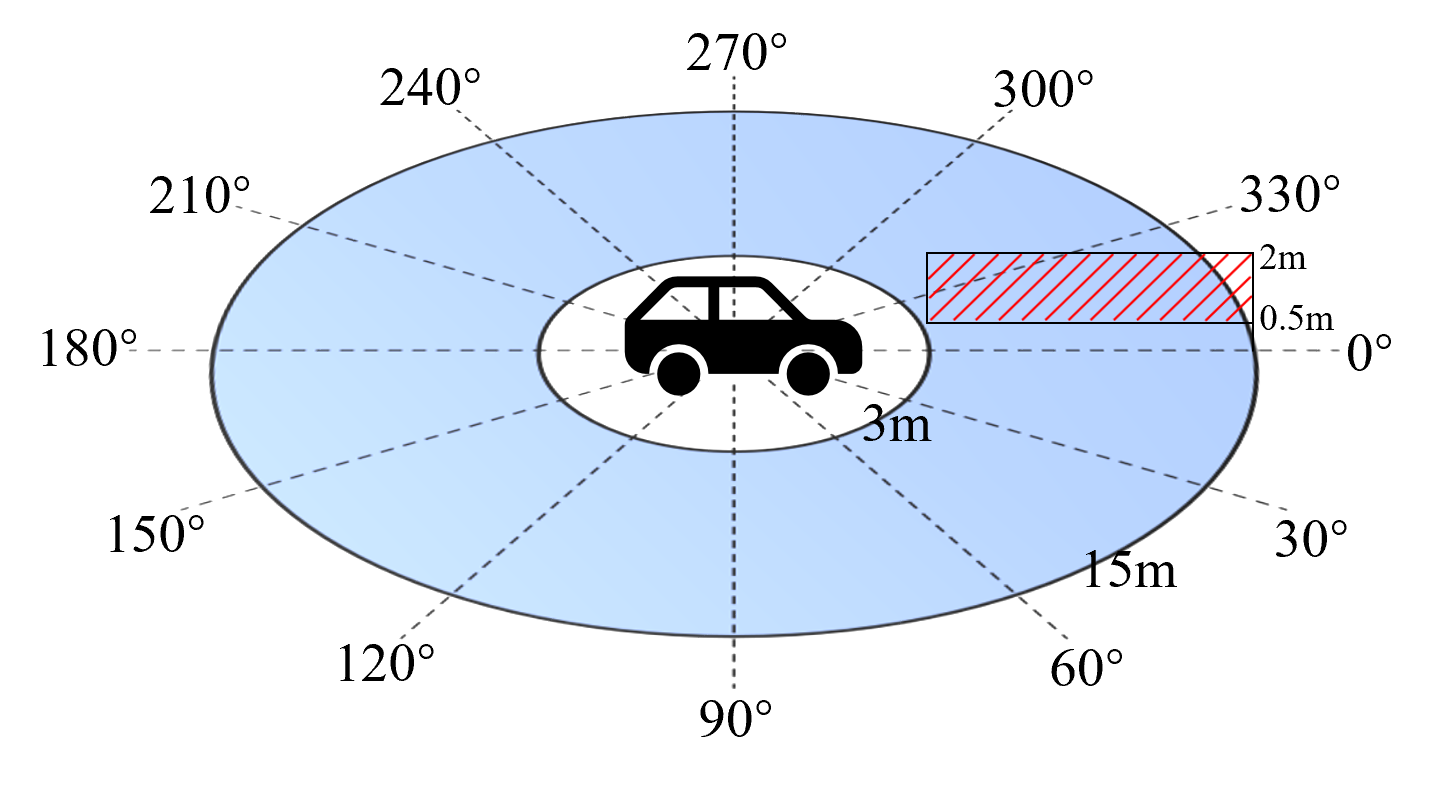}
    \caption{Camera position settings in Carla.}
    \label{fig:12}
\end{figure}

\subsection{Compared Attacks}
We provide detailed parameter settings of compared methods: APA~\cite{APA}, SPOO~\cite{SPOO}, APARATE~\cite{APARATE}, SAAM~\cite{SAAM}.

\begin{table}[!t]
\caption{Transformations distribution.}
\label{tab6}
  \centering
  \captionsetup{skip=3pt}
\resizebox{\linewidth}{!}{
  \begin{tabular}{ccc}
    \toprule
    Transformations & Parameters & Remark\\
    \midrule
    Rotation & $\pm 20^{\circ}$ & Camera Simulation\\
    Noise & $\pm 0.1$ & Random Noise\\
    Brightness & $\pm 0.2$ & Illumination\\
    Contrast & $[0.9, 1.1]$ & Camera Parameters\\
    Scale & $[0.25, 1.25]$ & Distance/Resize\\
    \bottomrule
  \end{tabular}
}
\end{table}

\begin{figure}[!t]
    \centering
    \includegraphics[width=\columnwidth]{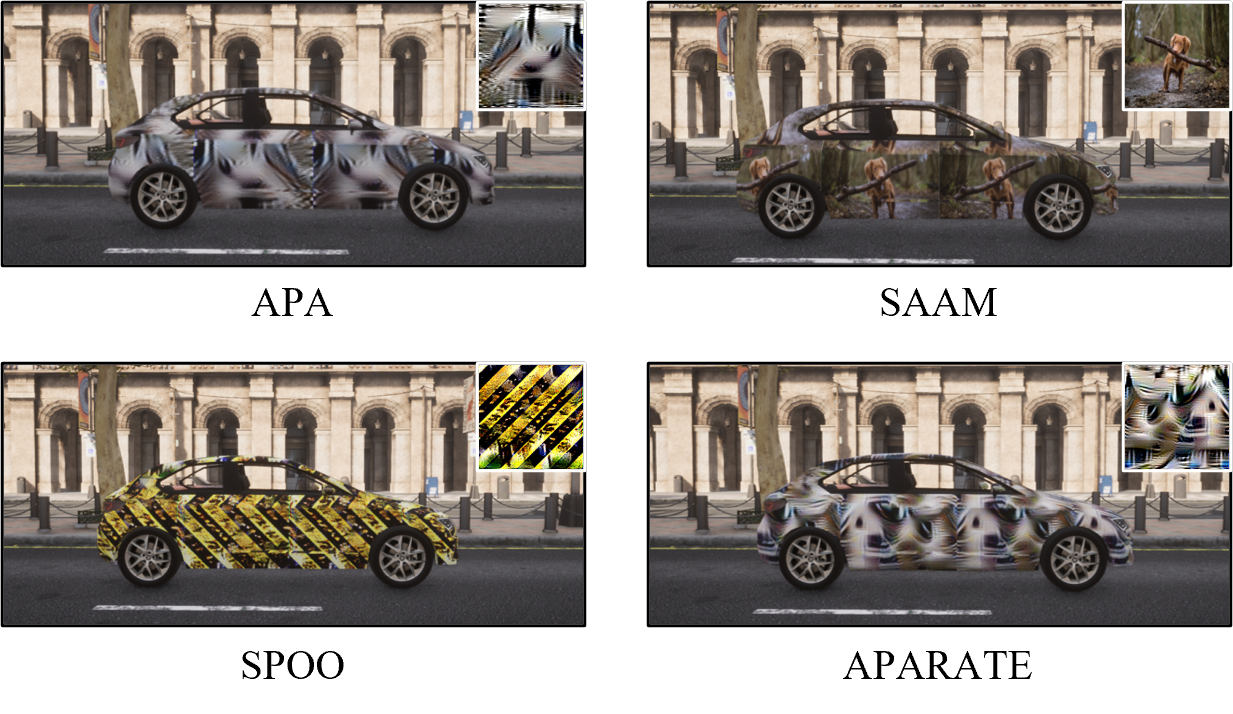}
    \caption{Adversarial cars with their initial patches (top right) in Carla.}
    \label{fig:14}
\end{figure}

\begin{figure*}[!t]
    \centering
    \includegraphics[width=\textwidth]{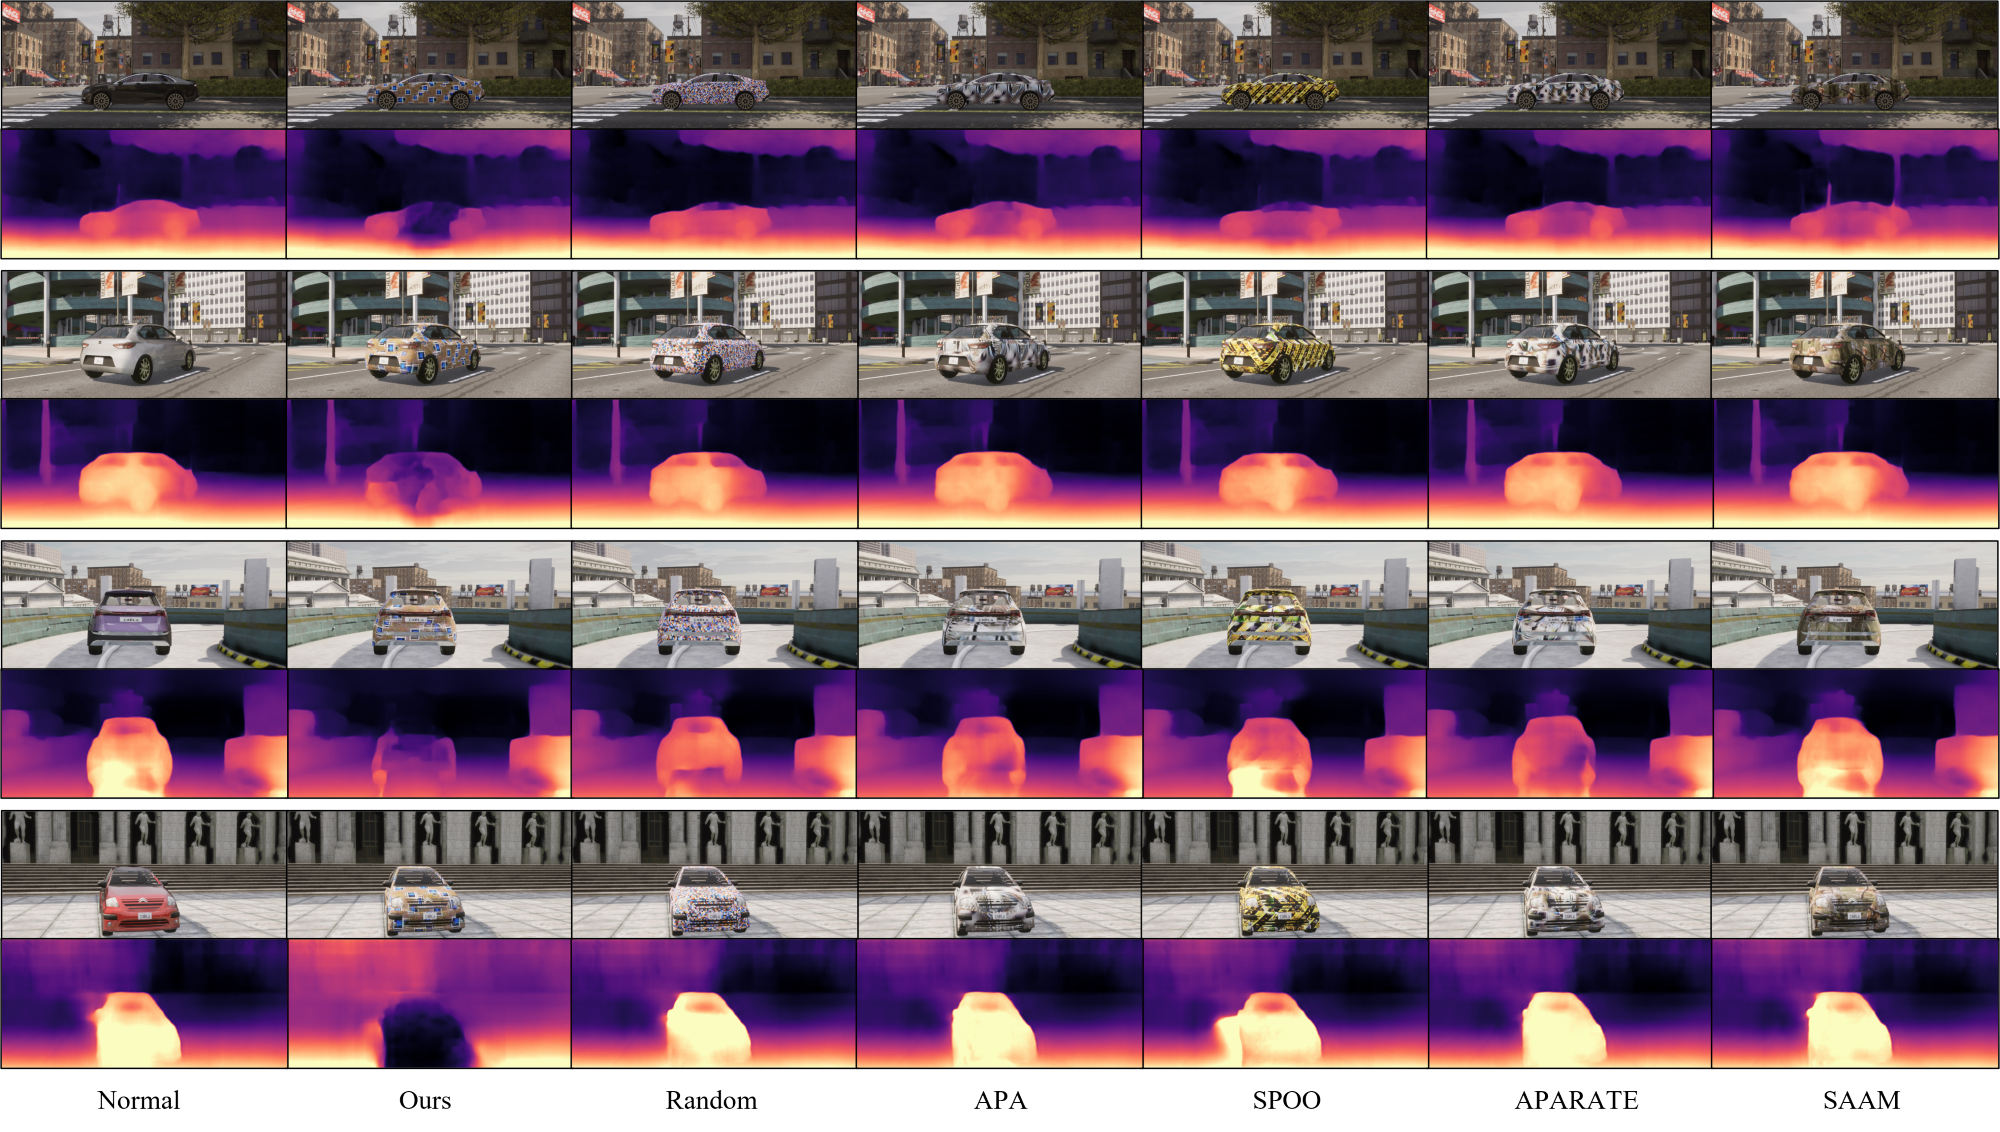}
    \caption{Comparisons of different attacks with various target vehicles and camera poses. The camera distance from the first row to the last is 9m, 7m, 5m, and 3m, respectively, and the camera viewpoints are lateral, lateral rear, rear, and front, respectively.}
    \label{fig:13}
\end{figure*}

\textbf{Patch-oriented attacks.} 
APA and SAAM are patch-oriented methods that fool MDE models into estimating an incorrect depth for the regions where the patterns are placed, independent of objects. APA is the first to attack MDE models in real scenes. SAAM leverages a semantic constraint to ensure the stealthiness of the generated adversarial patch. Data augmentation techniques used in the above methods mainly include rotation, brightness, contrast, etc. Detailed parameter settings are listed in Table~\labelcref{tab6}.

\textbf{Object-oriented attacks.} SPOO and APARATE are object-oriented methods expected to affect the depth estimation of the whole target region. SPOO is the first to consider stealth for attacking MDE models in real scenes. APARATE designs a penalized loss function to enlarge the affected region. We use the same transformations in Table~\labelcref{tab6}.
For the above four attacks, initial patches with the size of 512$\times$512 retrained on Monodepth2~\cite{monodepth2} and the corresponding adversarial images in Carla are shown in Figure~\labelcref{fig:14}.

\section{Evaluation Details}
\hspace{1em}\textbf{Various camera Poses and target vehicles.} We evaluate attack methods on Monodepth2 with various camera poses, for distance and rotation. Figure~\labelcref{fig:13} shows the attack performance of different attack methods on four target vehicles, at various distances and camera viewpoints. Our method outperforms the remaining attack methods on different target vehicles.

\textbf{Various weather conditions.} We evaluate attack methods on Monodepth2 under various weather conditions. Figure~\labelcref{fig:15} shows the attack performance on the Audi Etron under four weather conditions. Our method outperforms the remaining attack methods under various weather conditions.

\textbf{Various target objects.} We evaluate attack methods on pedestrians, trucks, and buses against Monodepth2. Figure~\labelcref{fig:16} shows the attack performance under default weather conditions. Considering the different sizes of the target objects, the texture size is correspondingly scaled by different factors.

\textbf{Real-world evaluations.} We provide detailed samples to show our camouflage texture performance in the real world. Figure~\labelcref{fig:17} shows that the adversarial car can deceive Monodepth2, regardless of viewpoints.

\begin{figure*}[!t]
    \centering
    \includegraphics[width=\textwidth]{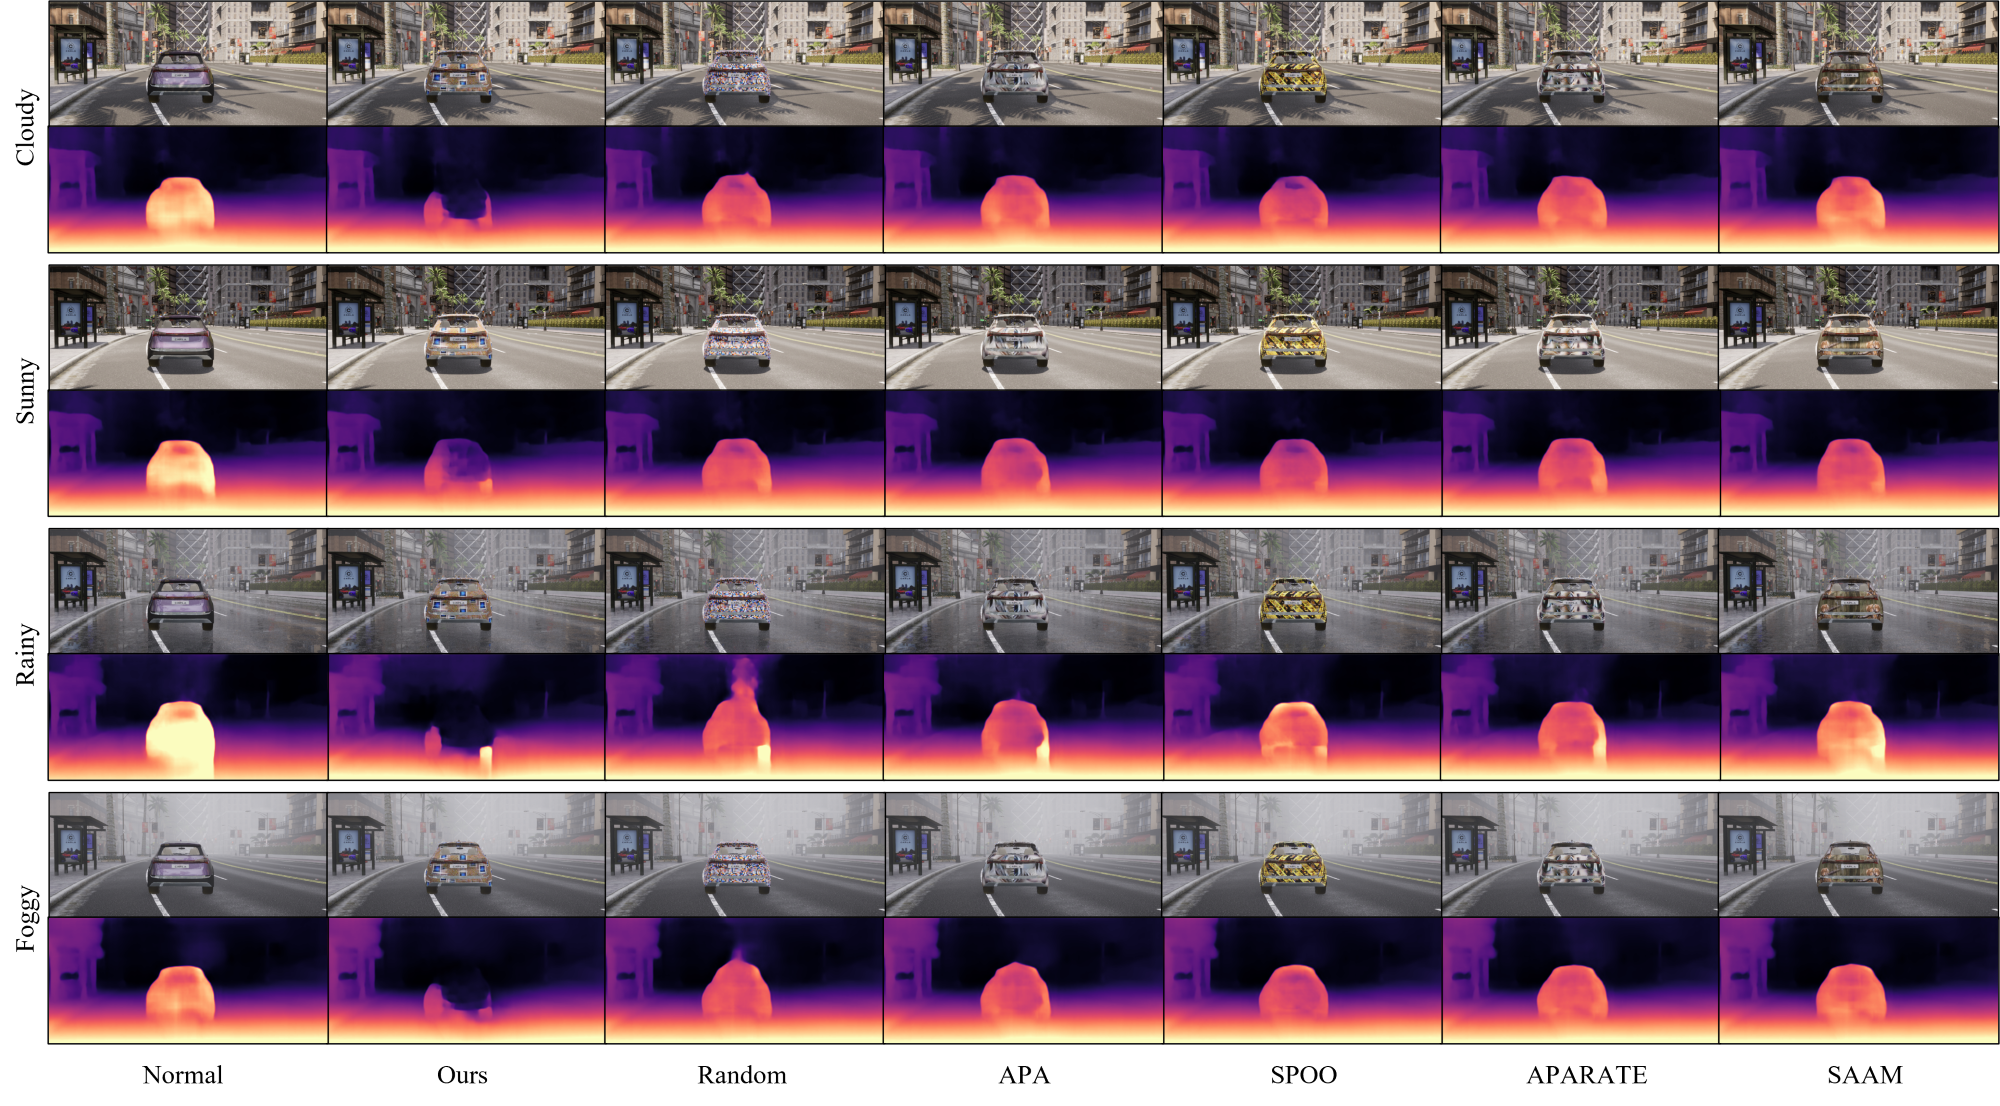}
    \caption{Comparisons of different attacks with various weather conditions: cloudy, sunny, rainy, and foggy. The camera viewpoint is the rear and the distance is 6m. }
    \label{fig:15}
\end{figure*}

\begin{figure*}[!t]
    \centering
    \includegraphics[width=\textwidth]{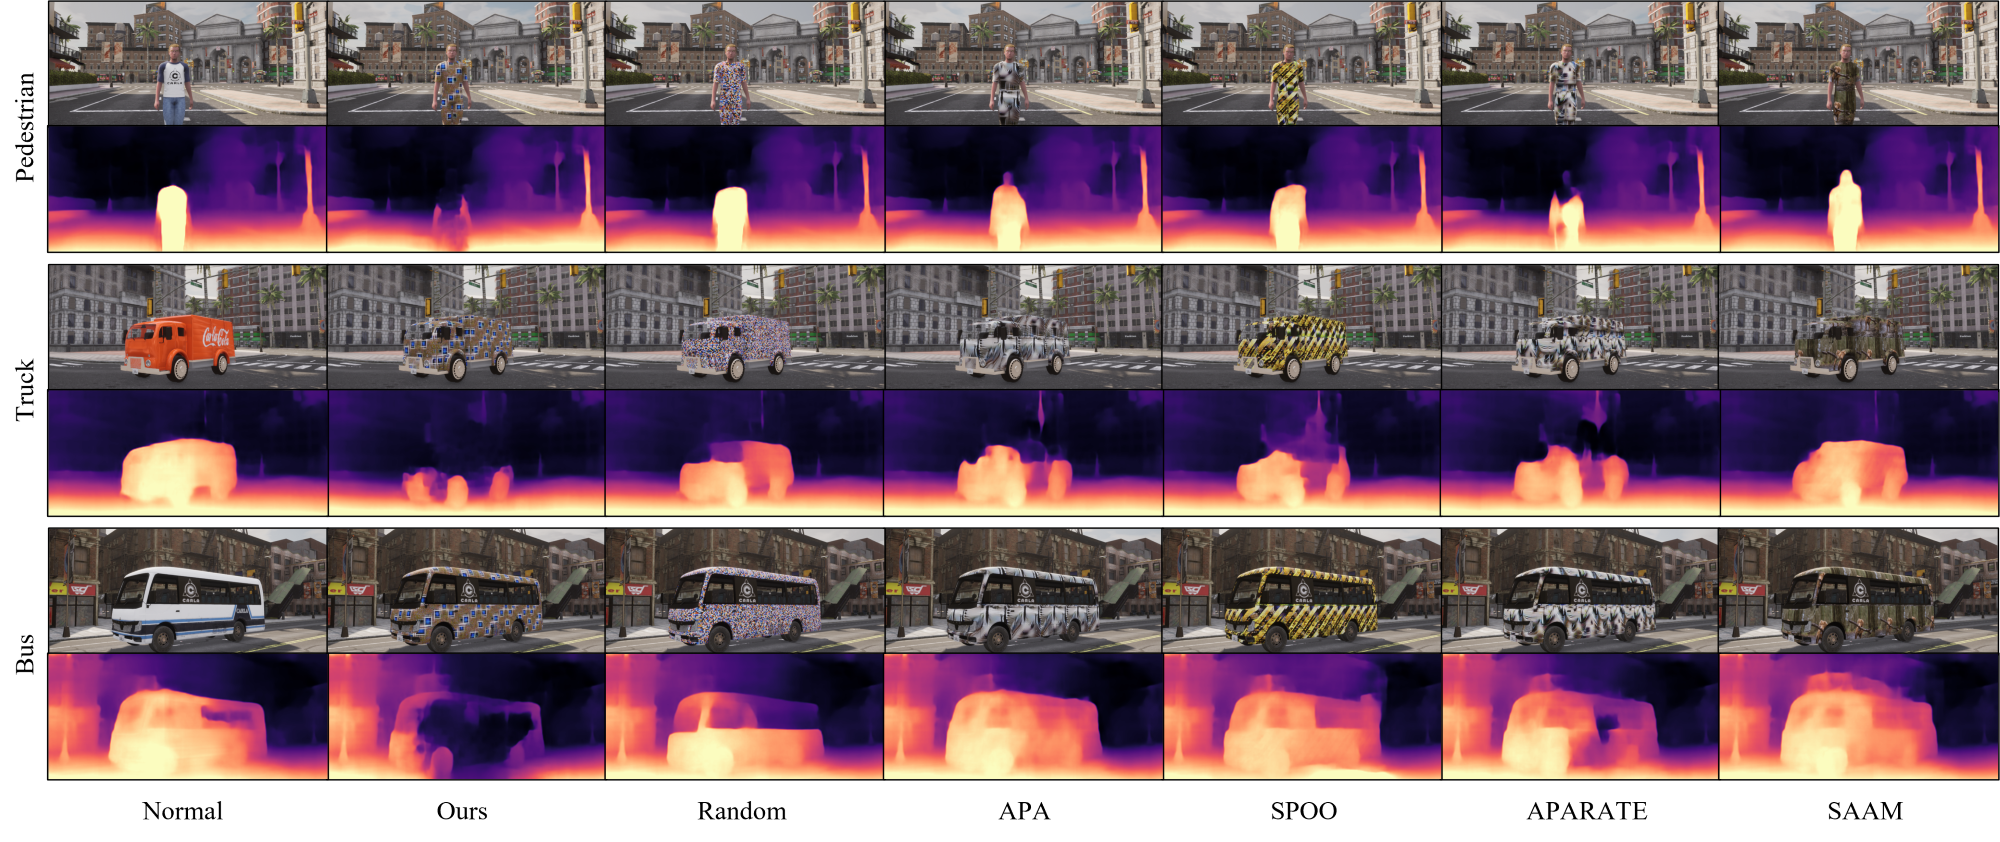}
    \caption{Comparisons of different attacks with various target objects: pedestrian, truck, and bus. Considering the different sizes of the target objects, the texture size is scaled by 0.5, 1.3, and 1.8, respectively.}
    \label{fig:16}
\end{figure*}

\begin{figure*}[!t]
    \centering
    \includegraphics[width=\textwidth]{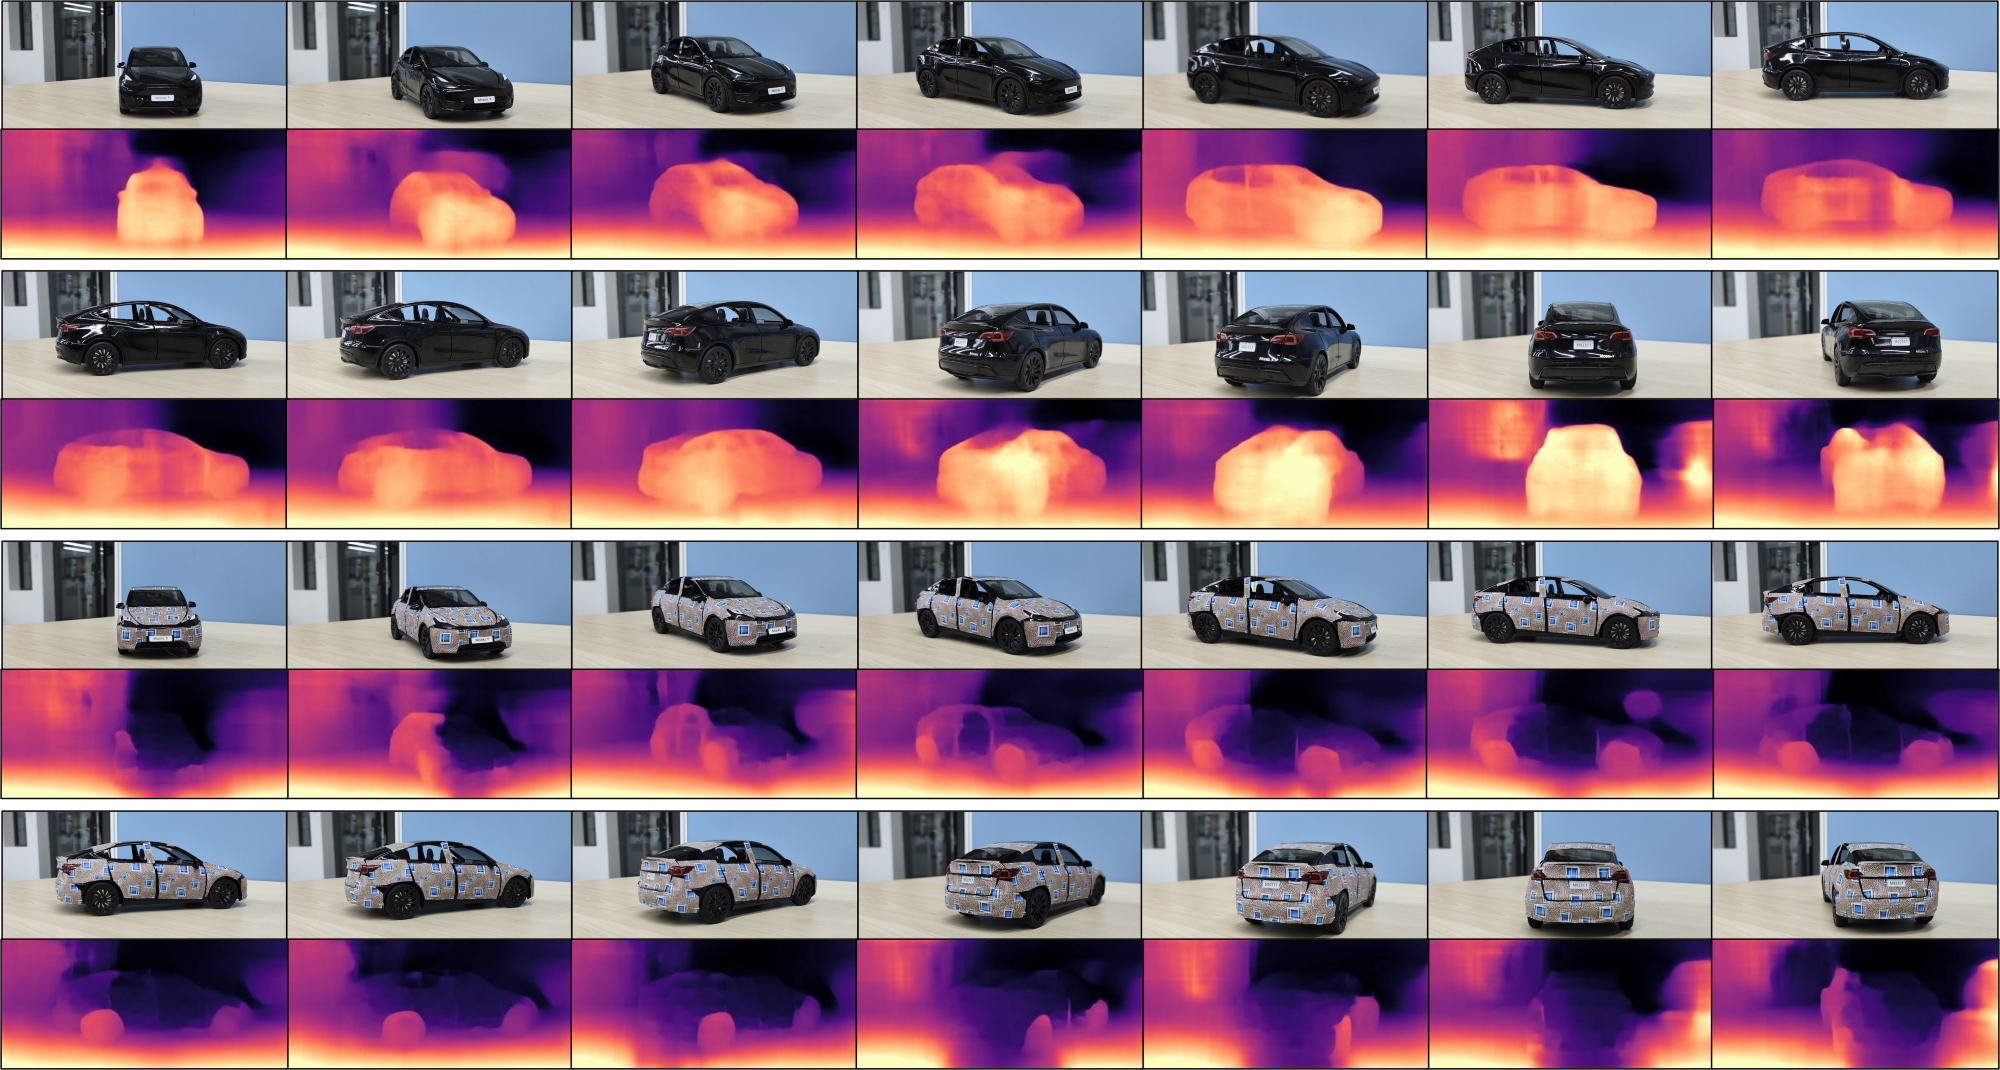}
    \caption{Real-world evaluations with normal and our adversarial scaled car models.}
    \label{fig:17}
\end{figure*}

\begin{figure*}[!t]
    \centering
    \includegraphics[width=\textwidth]{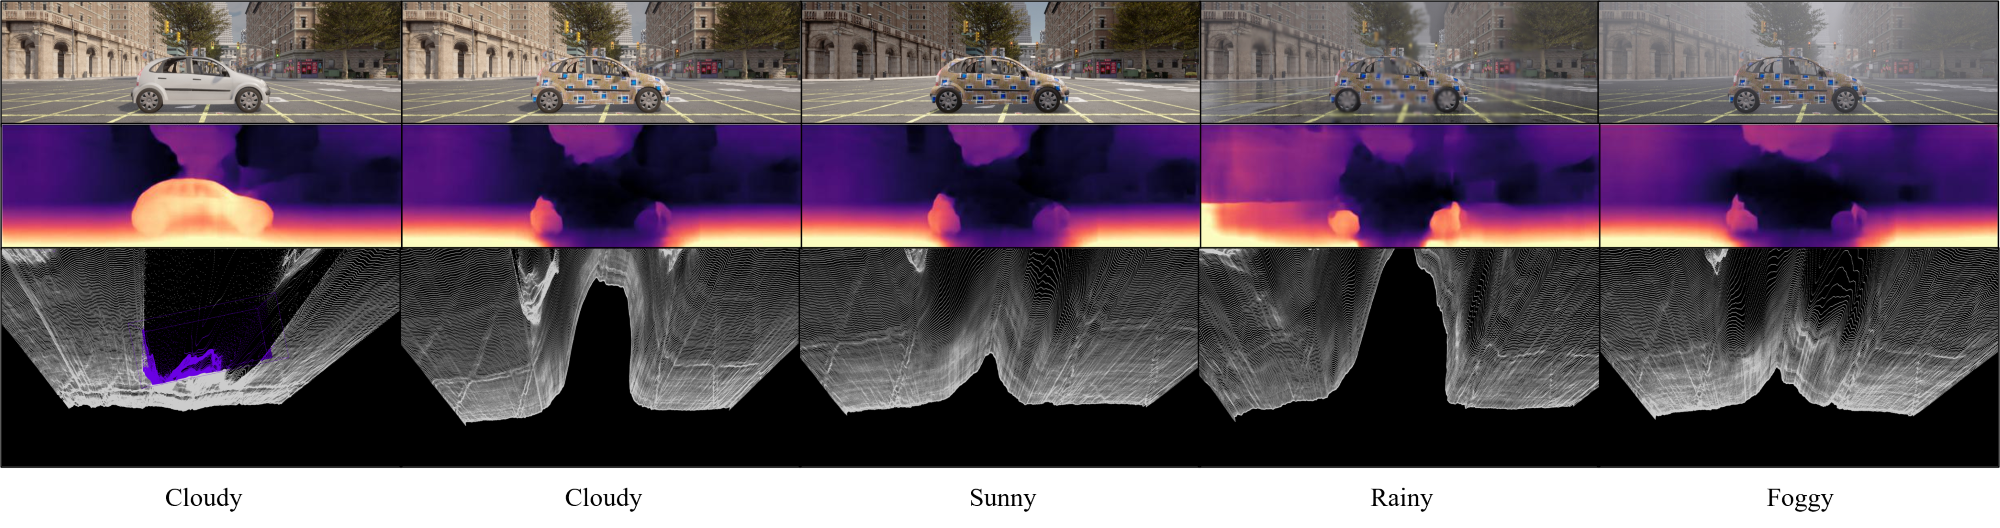}
    \caption{Our attack against 3D object detection with various weather conditions.}
    \label{fig:18}
\end{figure*}

\textbf{Impact on a downstream task.} Following the experiments in~\cite{SPOO}, we evaluate the impact of our attack on a point cloud-based 3D object detection model, PointPillars~\cite{PointPillars}, and use Detection Rate as the metric to evaluate our method on 3D object detection. We collect 8 videos with 331 frames in Carla, where the observer drives sideways from the target vehicle, simulating the scenario of an autonomous vehicle. The target vehicles are covered by normal or camouflage textures under the four preset weather mentioned above. As shown in Figure~\labelcref{fig:18}, the benign vehicle can be correctly detected with a 3D bounding box. In contrast, the pseudo-Lidar point cloud of the camouflaged vehicles is severely distorted, and camouflaged vehicles are not detected. Table~\labelcref{tab7} shows the detection rate of the normal vehicle and camouflaged vehicles detected under different weather conditions.

\begin{table}[!t]
\caption{Our attack against 3D object detection with various weather conditions. Values are detection rate.}
\label{tab7}
  \centering
  \captionsetup{skip=3pt}
\resizebox{\linewidth}{!}{
  \begin{tabular}{ccccc}
    \toprule
    \multirow{2}[3]{*}{Methods} & \multicolumn{4}{c}{Weather conditions}\\
\cmidrule{2-5}          & cloudy & sunny & rainy & foggy\\
    \midrule
    Normal & 82.18\% & 86.40\% & 80.66\% & 78.25\% \\
    \midrule
    Ours & 3.93\% & 5.74\% & 4.23\% & 2.72\% \\
    \bottomrule
  \end{tabular}
}
\end{table}
